# Supplementary material for: Quantitative Separation Logic - A Logic for Reasoning about Probabilistic Programs
Source: arXiv:1802.10467 source file (2018-11-26)
Supplement: Supplementary file 1 [file appendix-leftovers.tex]

\section{Quantitative Separation Logic (Leftovers)}

\blkcommentinline{Separating plus as first class citizen.}
\blkcommentinline{\atkb remove the following or move to appendix?}
\kbcommentinline{\atblk Yes, we can safely remove the following}
\begin{lemma}
       \label{lem:sepcon-unique-heap}
       Let $\ff$ be an expectation and $\preda$ be a predicate such that for every stack $\sk$ there is \emph{exactly one} heap $\hh'$ with $\iverson{\preda}(\sk,\hh') =1$.
       For every state $(\sk,\hh)$ where $\hh = \hh' \sepcon \restrictFunc{\hh}{\dom{\hh}\setminus\dom{\hh'}}$, we have
       \begin{equation*}
              (\iverson{\preda} \sepcon \ff)(\sk,\hh) \eeq  \iverson{\preda}(\sk,\hh') \cdot \ff\left(\sk, \restrictFunc{\hh}{\dom{\hh}\setminus\dom{\hh'}}\right)~.
       \end{equation*}
\end{lemma}
\begin{proof}
      We consider the cases $(\iverson{\preda} \sepcon \ff)(\sk,\hh) = 0$ and $(\iverson{\preda} \sepcon \ff)(\sk,\hh) \neq 0$. If we suppose $(\iverson{\preda} \sepcon \ff)(\sk,\hh) = 0$, then by definition
      $\iverson{\preda}(\sk,\hh_1) \cdot \ff(\sk,\hh_2) = 0$ for all $\hh_1, \hh_2$ with $\hh = \hh_1 \sepcon \hh_2$ and in particular for $\hh_1 = \hh'$ and $\hh_2 = \restrictFunc{\hh}{\dom{\hh}\setminus\dom{\hh'}}$. Now assume $(\iverson{\preda} \sepcon \ff)(\sk,\hh) \neq 0$ and let
      $\hh_1, \hh_2$ be heaps such that
      \begin{equation*}
             \iverson{\preda(\sk,\hh_1)} \cdot \ff(\sk,\hh_2) \eeq (\iverson{\preda} \sepcon \ff)(\sk,\hh)~.
      \end{equation*}
      Since $\iverson{\preda}(\sk,\hh_1) \cdot \ff(\sk,\hh_2) \neq 0$, we have $\iverson{\preda}(\sk,\hh_1) \neq 0$ and thus $\hh_1 =\hh'$ and $\hh_2 =  \restrictFunc{\hh}{\dom{\hh}\setminus\dom{\hh'}}$.
      \end{proof}
\begin{lemma}
        \label{lem:sepimp-unique-heap}
        Let $\ff$ be an expectation and $\preda$ be a predicate such that for every stack $\sk$ there is \emph{exactly one} heap $\hh'$ with $\iverson{\preda}(\sk,\hh') =1$.
        For every state $(\sk,\hh)$ where $\hh \disjoint \hh'$, we have
        \begin{equation*}
               (\iverson{\preda} \sepimp \ff)(\sk,\hh)  \eeq \ff(\sk, \hh \sepcon \hh')~.
        \end{equation*}
\end{lemma}
\begin{proof}
       Since there is exactly one $\hh'$ with $\iverson{\preda}(\sk,\hh') =1$, we have
       \begin{align*}
                     (\iverson{\preda} \sepimp \ff)(\sk,\hh)  &\eeq \inf_{\hh''} \left\{ \ff(\sk, \hh \sepcon \hh'') \mid \hh \disjoint \hh'', \iverson{\preda}(\sk,\hh'') =1  \right\} \\
                     &\eeq \ff(\sk, \hh \sepcon \hh')~.
       \end{align*}

\end{proof}

\subsection{Inference Rules (Hoare Logic)}
%\subsubsection{Frame Rule}
\paragraph{Frame Rule}
Given a program $\cc \in \hpgcl$ and a state $(\sk,\hh) \in \States$, we write $\toState{\configuration{\cc}{(\sk,\hh)}}{\abort}$ 
to denote that executing $\cc$ on $(\sk,\hh)$ leads to an abortion of the program. Furthermore we write $\configuration{\cc}{(\sk,\hh)}\nonTermination$ if $\cc$ does
not terminate on initial state $(\sk,\hh)$, and $\toState{\configuration{\cc}{(\sk,\hh)}}{(\sk',\hh')}$ if there is an execution of $\cc$ on $(\sk,\hh)$ that terminates in state $(\sk', \hh')$. \par
For a program $\cc$ and expectations $\fg,\ff \in \E$, the annotation $\hoare{\fg}{\cc}{\ff}$ is valid if and only if the following holds
for all $(\sk,\hh), (\sk',\hh') \in \States$:
\begin{itemize}
       \item If $\toState{\configuration{\cc}{(\sk,\hh)}}{\abort}$ or $\configuration{\cc}{(\sk,\hh)}\nonTermination$, then $\fg(\sk,\hh) = 0$.
       \item If $\toState{\configuration{\cc}{(\sk,\hh)}}{(\sk',\hh')}$, then $\fg(\sk,\hh) \leq \ff(\sk',\hh')$.
\end{itemize}
We say that expectation $\fh \in \E$ is \emph{locally independent} of program $\cc$, if
\begin{equation*}
        \toState{\configuration{\cc}{(\sk_1,\hh_1)}}{(\sk_2,\hh_2)}
        \qquad \text{implies that} \qquad
        \fh(\sk_1, \hh) ~{}={}~ \fh(\sk_2, \hh)
\end{equation*} for all heaps $\hh \in \Heaps$. \\
(Here is a proof of the frame property:  \\
\url{https://link.springer.com/content/pdf/10.1007\%2F3-540-45931-6_28.pdf})
\begin{lemma}[Frame Property]
\label{lem:frame-property}
       Suppose 
       \begin{align*}
             \notToState{\configuration{\cc}{(\sk,\hh_1)}}{\abort}
              \qquad \text{and} \qquad
               \toState{\configuration{\cc}{(\sk,\hh_1\sepcon \hh_2)}}{\configuration{\cc}{(\sk',\hh')}}~.
       \end{align*}
        Then there is $\hh_1'$ such that
        \begin{align*}
               \toState{\configuration{\cc}{(\sk,\hh_1)}}{\configuration{\cc}{(\sk',\hh_1')}} \qquad \text{and} \qquad \hh' \eeq \hh_1'\sepcon \hh_2~.
        \end{align*}
\end{lemma}
\begin{theorem}[Frame Rule]
The following inference rule is sound.
\begin{equation*}
       \infer{\hoare{\fg \sepcon \fh}{\cc}{\ff \sepcon \fh}}{\hoare{\fg}{\cc}{\ff}}~,
\end{equation*}
where $\fh$ is locally independent of $\cc$.
\end{theorem}
\begin{proof}
       Suppose the annotation $\hoare{\fg}{\cc}{\ff}$ is valid. That is, for all $(\sk,\hh), (\sk',\hh') \in \States$, we have:
       \begin{itemize}
              \item If $\toState{\configuration{\cc}{(\sk,\hh)}}{\abort}$ or $\configuration{\cc}{(\sk,\hh)}\nonTermination$, then $\fg(\sk,\hh) = 0$.
              \item If $\toState{\configuration{\cc}{(\sk,\hh)}}{(\sk',\hh')}$, then $\fg(\sk,\hh) \leq \ff(\sk',\hh')$.
       \end{itemize}
       Now let $(\sk,\hh) \in \States$ and let $\hh_1, \hh_2 \in \Heaps$ such that
       \begin{equation*}
              \fg(\sk,\hh_1) \cdot \fh(\sk,\hh_2) ~{}={}~ (\fg \sepcon \fh)(\sk,\hh)~.
       \end{equation*}
       We distinguish the cases $\toState{\configuration{\cc}{(\sk,\hh)}}{\abort}$, $\configuration{\cc}{(\sk,\hh)}\nonTermination$, and
       $\toState{\configuration{\cc}{(\sk,\hh)}}{(\sk',\hh')}$. \\ \\
       \emph{First case $\toState{\configuration{\cc}{(\sk,\hh)}}{\abort}$.} Then $\toState{\configuration{\cc}{(\sk,\hh_1)}}{\abort}$ (see Reynolds paper)
       and hence $\fg(\sk,\hh_1) \cdot \fh(\sk,\hh_2) = 0 \cdot \fh(\sk,\hh_2) = 0$ by assumption. \\ \\
       \emph{Second case $\configuration{\cc}{(\sk,\hh)}\nonTermination$.} This case is analogous to the first case since $\configuration{\cc}{(\sk,\hh)}
       \nonTermination$ implies that either 
       $\toState{\configuration{\cc}{(\sk,\hh_1)}}{\abort}$ or $\configuration{\cc}{(\sk,\hh_1)}\nonTermination$. \\ \\
       \emph{Third case $\toState{\configuration{\cc}{(\sk,\hh)}}{(\sk',\hh')}$.}
       If $\toState{\configuration{\cc}{(\sk,\hh_1)}}\abort$, then $\fg(\sk,\hh_1) = 0$ and therefore $\fg(\sk, \hh_1) \cdot \fh(\sk, \hh_2) = 0 \leq (\ff \sepcon \fh)(\sk',\hh')$.
       Now assume $\notToState{\configuration{\cc}{(\sk,\hh_1)}}{\abort}$. We have to show that 
       \begin{align*}
              \fg(\sk,\hh_1) \sepcon \fh(\sk,\hh_2) \leq (\ff \sepcon \fh)(\sk',\hh')~,
       \end{align*}
       which boils down to showing that there are $H_1, H_2 \in \Heaps$ such that $\hh' = H_1 \sepcon H_2$ with $\fg(\sk,\hh_1) \cdot \fh(\sk,\hh_2) \leq \ff(\sk',H_1) \cdot \fh(\sk', H_2)$.
       By the frame property (Lemma~\ref{lem:frame-property}), there is a $\hh_1'$ such that $\toState{\configuration{\cc}{(\sk,\hh_1)}}{(\sk',\hh_1')}$ and $\hh' = \hh_1' \sepcon \hh_2$. We can thereby take $H_1 = \hh_1'$ and $H_2 = \hh_2$ to
       obtain
       \begin{align*}
              \ff(\sk',H_1) \cdot \fh(\sk', H_2) &\eeq \ff(\sk',H_1) \cdot \fh(\sk, H_2)
              \tag{$\fh$ is locally independent of $\cc$} \\
              &~{}\geq~{} \fg(\sk,\hh_1) \cdot \fh(\sk, \hh_2)~.
              \tag{$H_2 = \hh_2$ and $\ff(\sk',H_1) \geq \fg(\sk,\hh_1)$ by assumption}
       \end{align*}
\end{proof}
\subsection{Various Lemmas}
\begin{lemma}
       \label{lem:two-replacements}
       For all arithmetic expressions over local variables $\ee_1,\ee_1',\ee_2,\ee_2'$ and all expectations $\ff$, we have
       \begin{align*}
              \phantom{\eeq}& \validpointer{\ee_1} \sepcon \left( \singleton{\ee_1}{\ee_1'} \sepimp \left(\validpointer{\ee_2}\sepcon \left( \singleton{\ee_2}{\ee_2'} \sepimp \ff \right) \right) \right) \\
             \eeq&\validpointer{\ee_1} \sepcon \validpointer{\ee_2} \sepcon \left(\left( \singleton{\ee_1}{\ee_1'} \sepcon \singleton{\ee_2}{\ee_2'} \right) \sepimp \ff \right) \\
                    &\quad +\iverson{\ee_1 = \ee_2} \cdot \left( \validpointer{\ee_2} \sepcon \left( \singleton{\ee_2}{\ee_2'} \sepimp \ff \right)  \right)~.
       \end{align*}
\end{lemma}
       \begin{proof}
           See Appendix~\ref{proof:lem:two-replacements}.
       \end{proof}
\begin{lemma}\label{lem:oplus-laws}
Separating plus $\oplus$ is commutative and associative.
\end{lemma}
\begin{proof}
Analogous to the proof of this lemma with respect to $\sepcon$.
\end{proof}

\section{Leftovers from wp}

\blkcommentinline{\atkb The following soundness theorem does not quite fit the probabilistic setting anymore, right?}
\kbcommentinline{\atblk Right. However, we could keep the proofs of the base cases to use the ideas in case we proof the probabilistic $\wpsymbol$ sound.}
\begin{theorem}[Soundness of $\wpsymbol$]
\label{thm:soundness-wp}
Let $\cc \in \hpgcl$, $(\sk,\hh) \in \States$, and $\ff\in \E$. Then the following holds:
\begin{enumerate}
       \item If $\toState{\configuration{\cc}{(\sk,\hh)}}{\abort}$ or $\configuration{\cc}{(\sk,\hh)}\nonTermination$, then
       \begin{equation*}
              \wp{\cc}{\ff}(\sk,\hh) \eeq 0~.
       \end{equation*}
       \item If $\notToState{\configuration{\cc}{(\sk,\hh)}}{\abort}$ and $\neg \left( \configuration{\cc}{(\sk,\hh)}\nonTermination \right)$, then
       \begin{equation*}
              \wp{\cc}{\ff}(\sk,\hh) \eeq \inf_{(\sk',\hh')} \setcomp{ \ff(\sk', \hh')}{\toState{\configuration{\cc}{(\sk,\hh)}}{\terminatedState{(\sk',\hh')}}}~.
       \end{equation*}
\end{enumerate}
\end{theorem}
\begin{proof}
By induction on the structure of a $\hpgcl$ program $\cc$. See Appendix~\ref{proof:thm:soundness-wp}.
\end{proof}
