# Supplementary material for: Quantitative Separation Logic - A Logic for Reasoning about Probabilistic Programs
Source: arXiv:1802.10467 source file (2018-11-26)
Supplement: Supplementary file 2 [file appendix-tree-height.tex]

\subsection{Full Proof for Expected Tree Height Example}

\begin{align*}
& \wp{c_{\textrm{rotate}}}{\Tree{x} \cdot \Path{x}} \\
\end{align*}

\begin{align*}
     & \wp{\texttt{rotateLeft}(x)}{\Tree{x} \cdot \Path{x}} \\
\eeq & \tag{Definition of \texttt{rotateLeft}} \\
     & \wp{\ASSIGNH{y}{x+1}\SEMI\ASSIGNH{z}{y}\SEMI\HASSIGN{y}{x}\SEMI\HASSIGN{x+1}{z}\SEMI\ASSIGN{x}{y}}{\Tree{x} \cdot \Path{x}} \\
\eeq & \tag{Table~\ref{table:wp}} \\
     & \wp{\ASSIGNH{y}{x+1}\SEMI\ASSIGNH{z}{y}\SEMI\HASSIGN{y}{x}\SEMI\HASSIGN{x+1}{z}}{\Tree{y} \cdot \Path{y}} \\
\eeq & \tag{Table~\ref{table:wp}} \\
     & \wp{\ASSIGNH{y}{x+1}\SEMI\ASSIGNH{z}{y}\SEMI\HASSIGN{y}{x}}{\validpointer{x+1} \sepcon \left(\singleton{x+1}{z} \sepimp \Tree{y} \cdot \Path{y}\right)} \\
\eeq & \tag{Table~\ref{table:wp}} \\
     & \wp{\ASSIGNH{y}{x+1}\SEMI\ASSIGNH{z}{y}}{\validpointer{y} \sepcon \left(\singleton{y}{x} \sepimp \validpointer{x+1} \sepcon \left(\singleton{x+1}{z} \sepimp \Tree{y} \cdot \Path{y}\right)\right)} \\
\eeq & \tag{Table~\ref{table:wp}, Lemma~\ref{lem:wand-reynolds}} \\
     & \wp{\ASSIGNH{y}{x+1}}{\sup_{v \in \Ints} \colon \containsPointer{y}{v} \cdot \left(\validpointer{y} \sepcon \left(\singleton{y}{x} \sepimp \validpointer{x+1} \sepcon \left(\singleton{x+1}{v} \sepimp \Tree{y} \cdot \Path{y}\right)\right)\right)} \\
\eeq & \tag{Table~\ref{table:wp}, Lemma~\ref{lem:wand-reynolds}} \\
     & \sup_{u,v \in \Ints} \colon \containsPointer{x+1}{u} \cdot \containsPointer{u}{v} \cdot (\validpointer{u} \sepcon (\singleton{u}{x} \sepimp \validpointer{x+1} \sepcon (\singleton{x+1}{v} \\
     & \qquad \sepimp \Tree{u} \cdot \Path{u}))) \\
\eeq & \tag{$\containsPointer{\alpha}{\beta} \cdot (\validpointer{\alpha} \sepcon f) = \singleton{\alpha}{\beta} \sepcon f$} \\
     & \sup_{u,v \in \Ints} \colon \containsPointer{x+1}{u} \cdot \singleton{u}{v} \sepcon (\singleton{u}{x} \sepimp \validpointer{x+1} \sepcon (\singleton{x+1}{v} \\
     & \qquad \sepimp \Tree{u} \cdot \Path{u}))) \\
\end{align*}

\begin{align*}
     & \wp{\texttt{rotateRight}(x)}{\Tree{x} \cdot \Path{x}} \\
\eeq & \tag{Table~\ref{table:wp}} \\
     & \wp{\ASSIGNH{y}{x}\SEMI\ASSIGNH{z}{y + 1}\SEMI\HASSIGN{y+1}{x}\SEMI\HASSIGN{x}{z}\SEMI\ASSIGN{x}{y}}{\Tree{x} \cdot \Path{x}} \\
\eeq & \tag{Table~\ref{table:wp}} \\
     & \wp{\ASSIGNH{y}{x}\SEMI\ASSIGNH{z}{y + 1}\SEMI\HASSIGN{y+1}{x}\SEMI\HASSIGN{x}{z}}{\Tree{y} \cdot \Path{y}} \\
\eeq & \tag{Table~\ref{table:wp}} \\
     & \wp{\ASSIGNH{y}{x}\SEMI\ASSIGNH{z}{y + 1}\SEMI\HASSIGN{y+1}{x}}{\validpointer{x} \sepcon (\singleton{x}{z} \sepimp \Tree{y} \cdot \Path{y})} \\
\eeq & \tag{Table~\ref{table:wp}} \\
     & \wp{\ASSIGNH{y}{x}\SEMI\ASSIGNH{z}{y + 1}}{\validpointer{y+1} \sepcon (\singleton{y+1}{x} \sepimp \validpointer{x} \sepcon (\singleton{x}{z} \sepimp \Tree{y} \cdot \Path{y}))} \\
\eeq & \tag{Table~\ref{table:wp}, Lemma~\ref{lem:wand-reynolds}} \\
     & \wp{\ASSIGNH{y}{x}}{\sup_{b \in \Ints}\mydot\containsPointer{y+1}{b} \cdot (\validpointer{y+1} \sepcon (\singleton{y+1}{x} \sepimp \validpointer{x} \sepcon (\singleton{x}{b} \sepimp \Tree{y} \cdot \Path{y})))} \\
\eeq & \tag{Table~\ref{table:wp}, Lemma~\ref{lem:wand-reynolds}} \\
     & \sup_{a,b \in \Ints}\mydot\containsPointer{x}{a} \cdot \containsPointer{a+1}{b} \cdot (\validpointer{a+1} \sepcon (\singleton{a+1}{x} \sepimp \validpointer{x} \sepcon (\singleton{x}{b} \\
     & \qquad \sepimp \Tree{a} \cdot \Path{a}))) \\
\eeq & \tag{$\containsPointer{\alpha}{\beta} \cdot (\validpointer{\alpha} \sepcon f) = \singleton{\alpha}{\beta} \sepcon f$} \\
     & \sup_{a,b \in \Ints}\mydot\containsPointer{x}{a} \cdot (\singleton{a+1}{b} \sepcon (\singleton{a+1}{x} \sepimp \validpointer{x} \sepcon (\singleton{x}{b} \\
     & \qquad \sepimp \Tree{a} \cdot \Path{a}))) \\
\end{align*}
