# Supplementary material for: Quantitative Separation Logic - A Logic for Reasoning about Probabilistic Programs
Source: arXiv:1802.10467 source file (2018-11-26)
Supplement: Supplementary file 4 [file appendix-operational-semantics.tex]

% !TEX root = ./main.tex

\subsection{Missing Definitions in Section~\ref{sec:operational}}
\label{app:operational-definitions}

\begin{definition}
        The \emph{GMC of a GMDP $\Mdp = (\OpStates,\OpActions,\ExecSymbol,\OpInit, \Target,\OpRew)$ induced by a scheduler $\Scheduler$} is given by
  \begin{align*}
     \MC{\Mdp}{\Scheduler} \eeq
     (\OpStates^{+},\{0\},\ExecSymbol',\OpInit, \PathsFromTo{\Mdp}{\OpInit},\OpRew')~,
  \end{align*}
  where, for $\vec{s} = s_1 s_2 \ldots s_n \in \OpStates^{+}$, we have
  \[ (\vec{s},0,p,\vec{s} \, s_{n+1}) \in \ExecSymbol' 
          ~\text{iff}~ (s_n,\Scheduler(\vec{s}), p, s_{n+1}) \in \ExecSymbol~.
  \]
  Moreover, for $\vec{s} = s_1 \ldots s_n \in \PathsFromTo{\Mdp}{\OpInit}$, we have
  $\OpRew'(\vec{s}) = \OpRew(s_n)$.
    \hfill$\triangle$
\end{definition}
